# Supplementary material for: Neural networks-based variationally enhanced sampling
Source: arXiv:1904.01305 ancillary file (2019-09-23)
Supplement: Supplementary file 1 [file supporting-information.pdf]

# Supplementary Information for

## Neural network based variationally enhanced sampling

**Luigi Bonati, Yue-Yu Zhang and Michele Parrinello**

**Michele Parrinello**
**E-mail: parrinello@phys.chem.ethz.ch**

### This PDF file includes:

Supplementary text
Figs. S1 to S5

## Supporting Information Text

### 1. Wolfe-Quapp potential

**A. PLUMED input file.** First we report an example of a PLUMED input file used to carry out the calculations with the modified version of the PLUMED2.

```
p: POSITION ATOM=1

DEEP_VES ...
LABEL=nn
ARG=p.x                 #CVs
NODES=48,24,12          #NN architecture
OPTIM=ADAM              #Optimizer (default:ADAM)
ACTIVATION=RELU         #Activation function (default:RELU)
GRID_MIN=-3.            #Grid settings (for numerical integration)
GRID_MAX=3.
GRID_BIN=50
TEMP=1.                 #Temperature
AVE_STRIDE=500          #Iteration lenght in MD steps
PRINT_STRIDE=1000       #Print stride (in iterations)
TARGET_STRIDE=1         #Target distribution update (in iterations)
GAMMA=10                #Well-tempered factor
LRATE=0.001             #Learning rate
TAU_KL=50000            #Scale on which the approximated KL is computed (in iterations)
DECAY=5000              #Decay time for the learning rate (in iterations)
ADAPTIVE_DECAY=0.5      #Threshold for KL (\epsilon)
... DEEP_VES
```

**B. Robustness of DEEP-VES with respect to the parameters.** We examined the behaviour of DEEP-VES with respect to the parameters used for the optimization scheme. We measured the root mean square errror (RMSE) between the FES learnt by DEEP-VES and the reference obtained by numerical integration of the model. Each simulations was run for $1 \cdot 10^8$ steps, corresponding to $2 \cdot 10^5$ iterations. The simulations were carried out with the following reference parameters: a KL divergence timescale of $5 \cdot 10^4$ iterations, $\epsilon = 0.5$, a learning rate decay equal to $5 \cdot 10^3$ iterations and employing a NN with three hidden layers and 48,24,12 nodes per layer. For every parameter 8 simulations with different seeds were performed, and the mean and the standard deviation of the RMSE were computed. In addition we report how many iterations were needed to converge to a static bias.

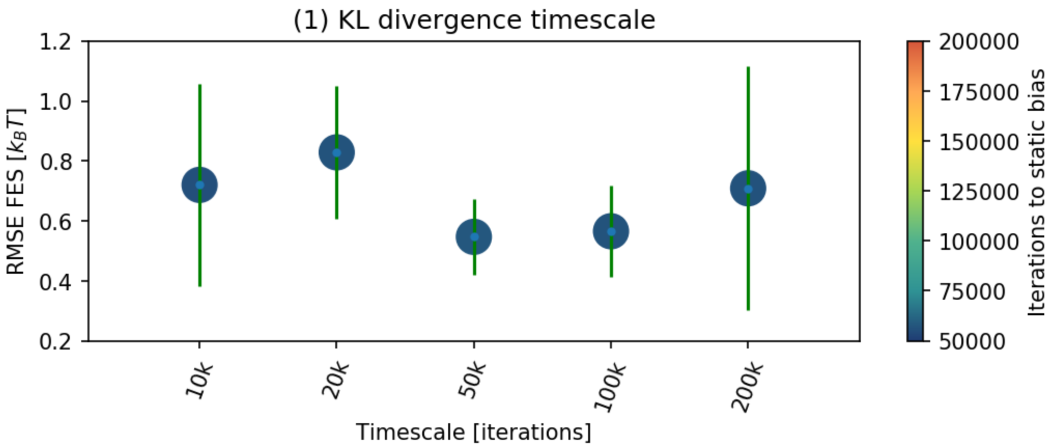


First we examined the impact of the timescale over which the KL divergence is evaluated with an exponentially decaying average, in figure (1). All the RMSE errors are below 1 $k_BT$. This timescale should be chosen such that the system is ergodic in such period of time, and thus will depend on the choice of the CVs as discussed in the main text. Choosing it as a fraction of the entire simulation (from a tenth to half of the simulation length) will lead to a good estimator for the KL, although it does not affect much the convergence speed.

Then we report the results obtained by changing the KL threshold $\epsilon$, below which the learning rate is exponentially decreased until it is practically zero. Figure (2) exemplifies the trade-off between speed and accuracy of the two phases, namely the

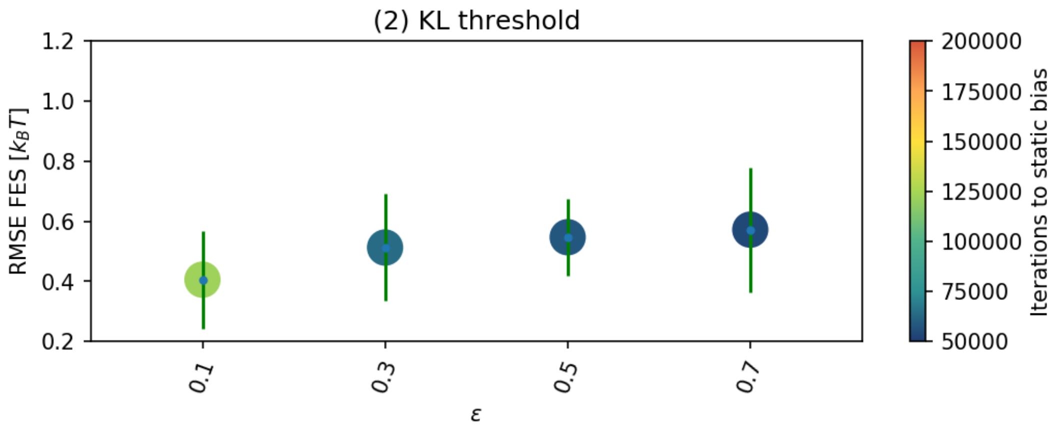


exploratory one and the subsequent slowing down of the optimization. Using a low threshold for the KL allows the NN to learn a better representation of the FES, but the price that needs to be paid is in the number of iterations. On the other hand, using a less stringent $\epsilon$ allows obtaining quickly a static bias, with only a small cost in terms of the accuracy.

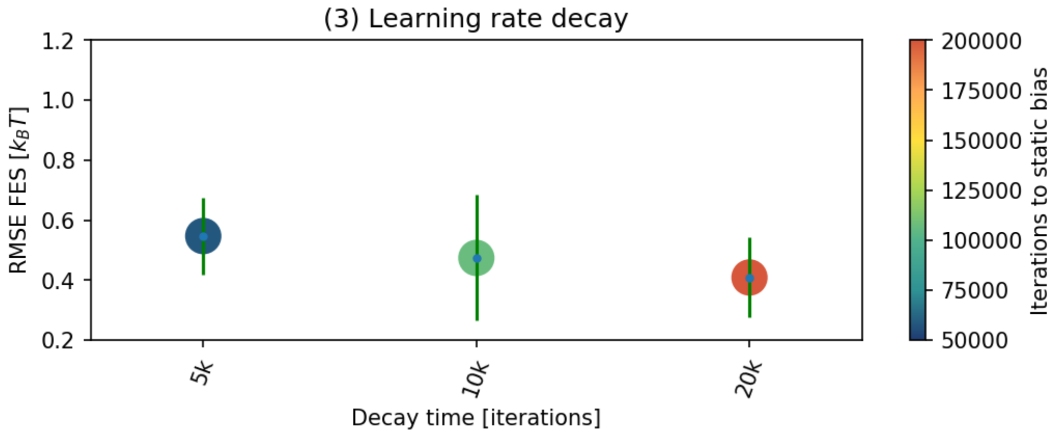


The next figure (3) shows the effect of the learning rate decay on the accuracy of the FES. Here a similar argument applies: the slower the decrease of the optimization the better the result will be. Nevertheless, even with a smaller decay we are able to get a good result. Care must be taken in the case of sub-optimal CVs, since choosing a too fast decay might lead to get stuck in some minimum.

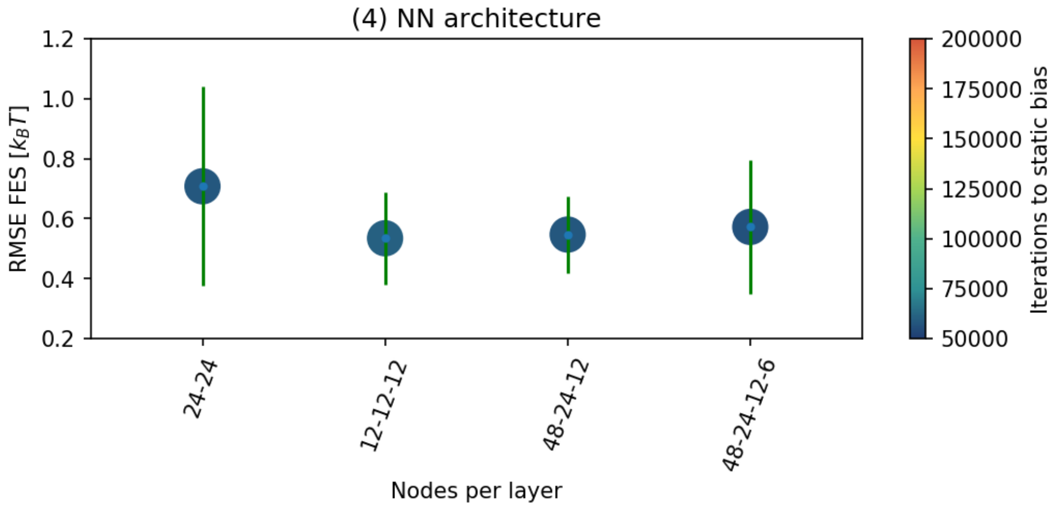

Last, we assessed the performance of DEEP-VES with respect to different architectures of the neural network, going from two to four layers, reported in figure (4). We obtain similar results for the different number of nodes. As in the the previous cases the choice should be thus motivated by a trade-off between the accuracy and the number of parameters of the network. We chose to use the 48-24-12 NN since it allowed to learn the bias of different kind of systems and FES dimensionalities.

As a final comment we would like to remember that the spirit of DEEP-VES is to use the expressivity of NN to quickly get a good representation of the bias potential which can be used as a static bias and subsequently refine the representation with a simple reweighting procedure. To reach this aim we do not need a perfect bias, and even an approximate one will work. In all the tests performed here the RMSEs were always below 1 $k_B T$. Therefore DEEP-VES is robust with respect to parameters used for the optimization scheme, as long as they are chosen in a reasonable range.

**C. Slowing down of the learning.** In figure S1 we compare the RMSE of the FES learned by DEEP-VES with the one obtained with the standard VES. The parameters are the same reported in the input file in 1A.

In the case of sub-optimal CVs, we find that the standard VES struggle to converge, even after a long simulation time. On the other hand, decreasing the learning rate according to the KL divergence with the target distribution on a characteristic timescale allows for quickly reaching an accurate value, which can be further improved with the umbrella-sampling like reweight (see fig. 2 of main text). For this reason we believe that also the VES could benefit from this feature.

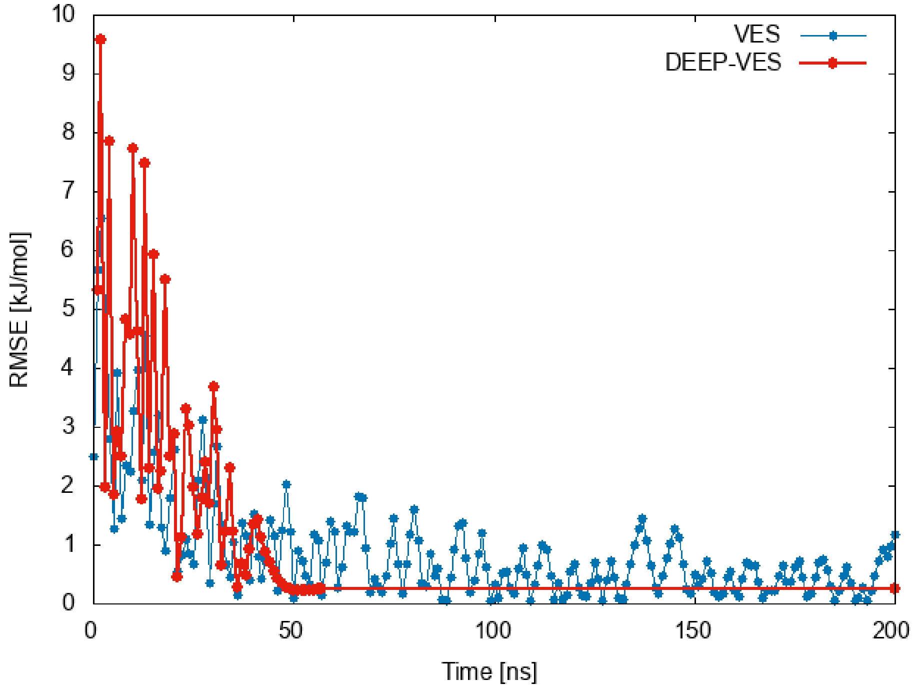


**Fig. S1.** RMSE of the FES learned by VES and DEEP-VES for the Wolfe-Quapp model.

## 2. Alanine dipeptide

In figure S2 we report the evolution of the CVs for a simulation of Ala2. The bias is defined in terms of $\phi$ and $\psi$. Since this is a good set of CVs, the NN quickly learns a good representation of the bias, which allows for an ergodic sampling of the well-tempered distribution. This is also proven by the fact that when the bias becomes static the transition rate remains similar to the first phase, since all the slow degrees of freedom are accounted for.

## 3. Alanine tetrapeptide

The alanine tetrapeptide simulation is carried out biasing the 6 diedhral angles.

**A. Monte Carlo integration.** Monte Carlo (MC) sampling is applied in high dimensional CV spaces to calculate the expectation value over the target distribution where numerical integration is expansive or unfeasible. Points following the target distribution in eq. 7 are generated by the Metropolis-Hastings algorithm. The desired distribution $p(s)$ could be calculated directly form the neural network potential $V(s)$, which follows

$$p(s) = e^{\frac{\beta}{\gamma-1}V(s)} / \int ds e^{\frac{\beta}{\gamma-1}V(s)}$$

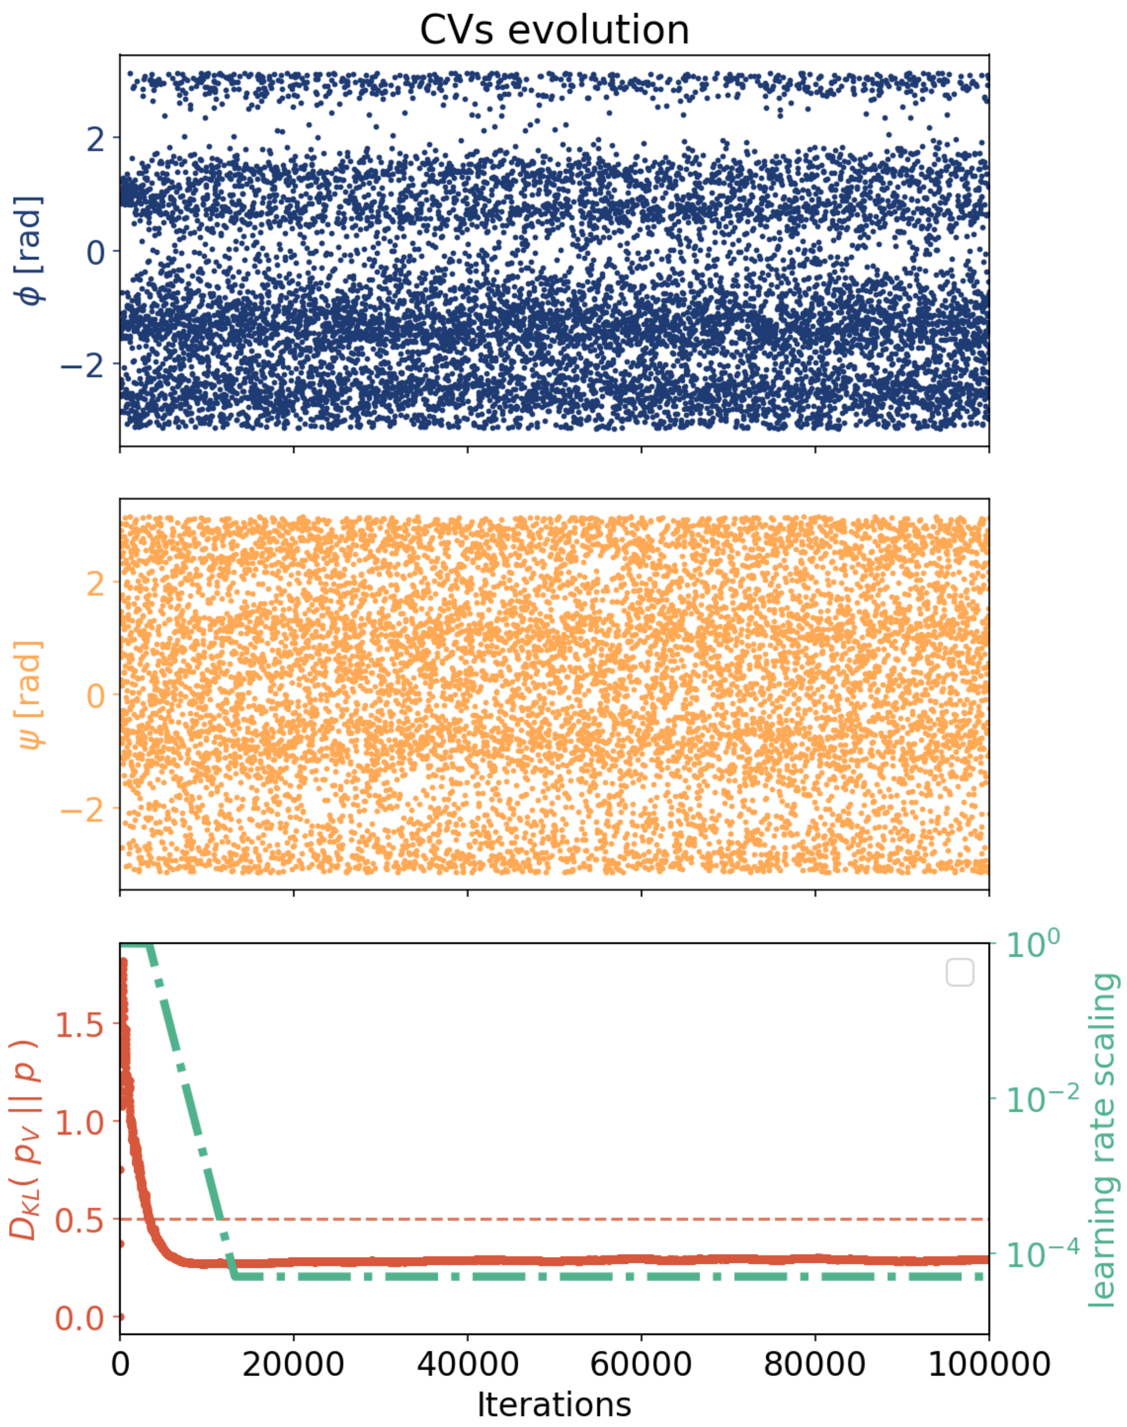


**Fig. S2.** Alanine dipeptide simulation. First and second panel: collective variables evolution in the simulation employing the DEEP-VES. Third panel: KL divergence and learning rate scaling with respect to its initial value. After 12 ns the simulations proceeds with a static bias potential.

Because only the ratio of $p(s')/p(s)$ is taken into account in the Metropolis algorithm, the integration of the denominator of $p(s)$ is neglected in the calculation. The number of MC points generated for studying alanine tetrapeptide with six CVs is $2 \cdot 10^4$, with a normalized root mean square error of the gradients less than 0.1%.

**B. CV evolution.** First we show the CVs evolution in fig. S3, together with the learning rate scaling. The system quickly reaches a diffusive behaviour in all the biased CVs, and is worth to note that the transition rate is unaffected also in the static bias regime.

**C. Accuracy of the FES.** In order to assess the accuracy of the results, we compare the reweighted free energy surfaces with the ones obtained with metadynamics and its parallel-bias variant. The former is carried out biasing only the three angles $\{\phi_1, \phi_2, \phi_3\}$. The latter applies multiple one-dimensional potentials over all the six $\{\phi_1, \phi_2, \phi_3\}$ angles. For both cases the Gaussian parameters are sigma equal to 0.35, initial height of 1.2 kJ/mol and biasfactor equal to 10. In figure S4 the projections on the pairs $\{\phi_1, \phi_2\}$ and $\{\phi_1, \psi_1\}$ are shown.

## 4. Silicon crystallization

In fig. S5 we report the CV evolution, together with the scaling of the learning rate, in order to show the transition rate in the different parts of the simulation.

## 5. Data sharing

The data used to produce the results of the paper will be uploaded on the Materials Cloud repository (https://archive.materialscloud.org/).

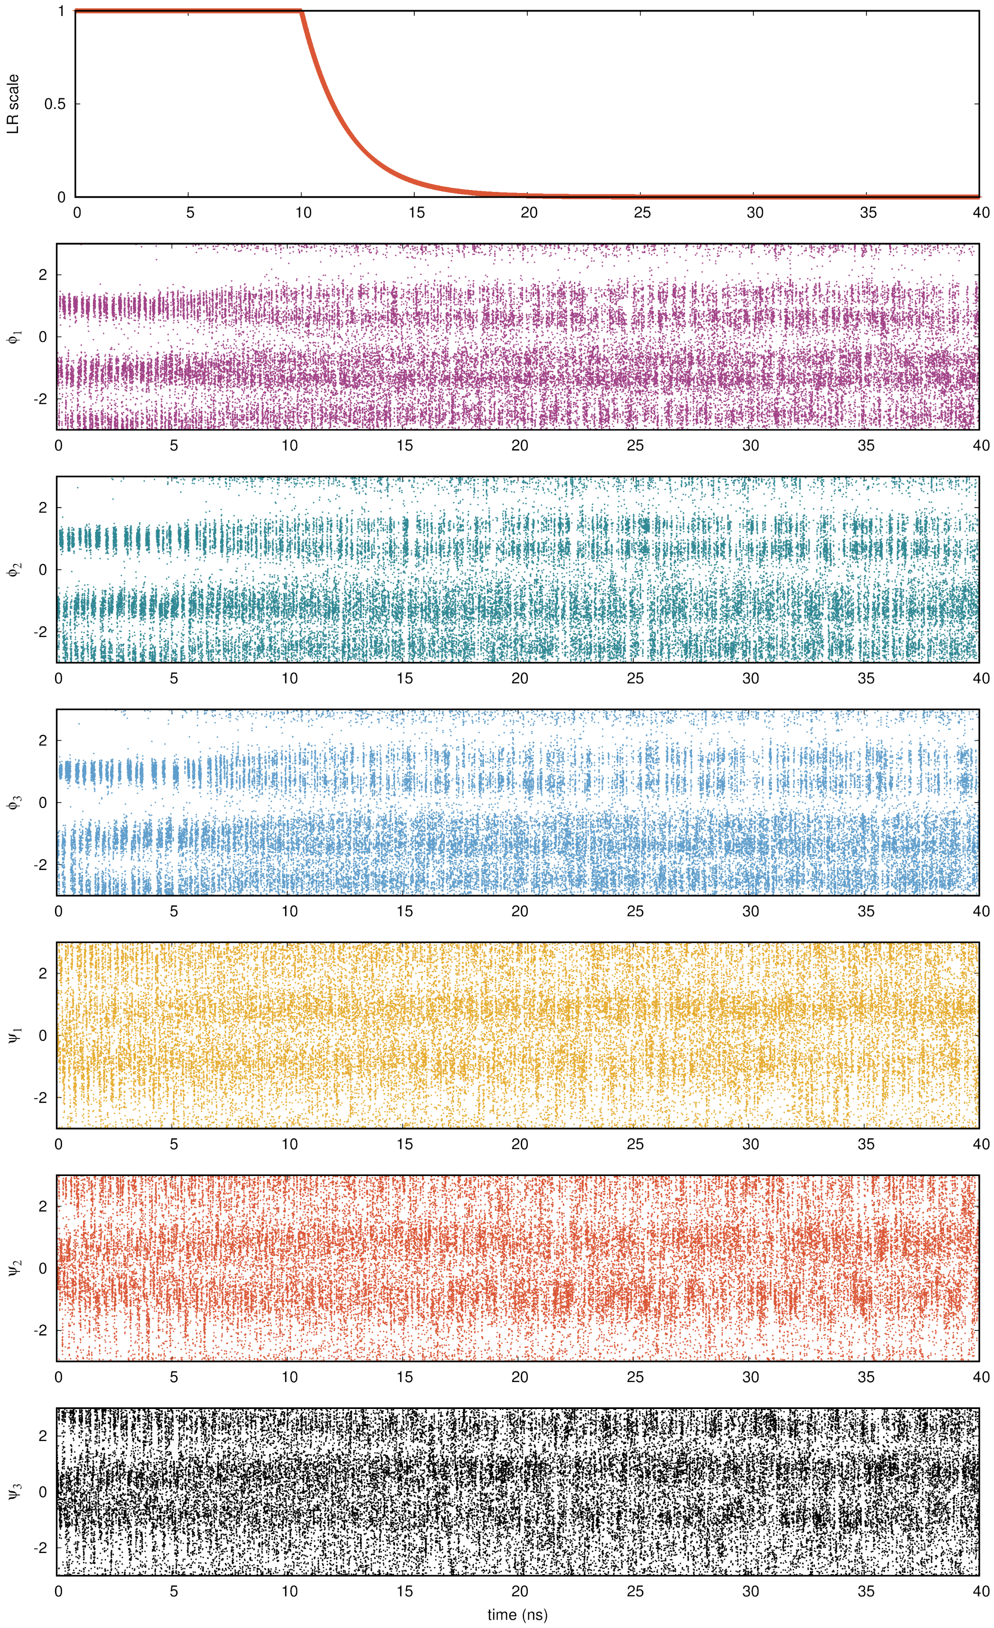


**Fig. S3.** Alanine dipeptide simulation. Top panel: learning rate scaling. Lower panels: Collective variables evolution.

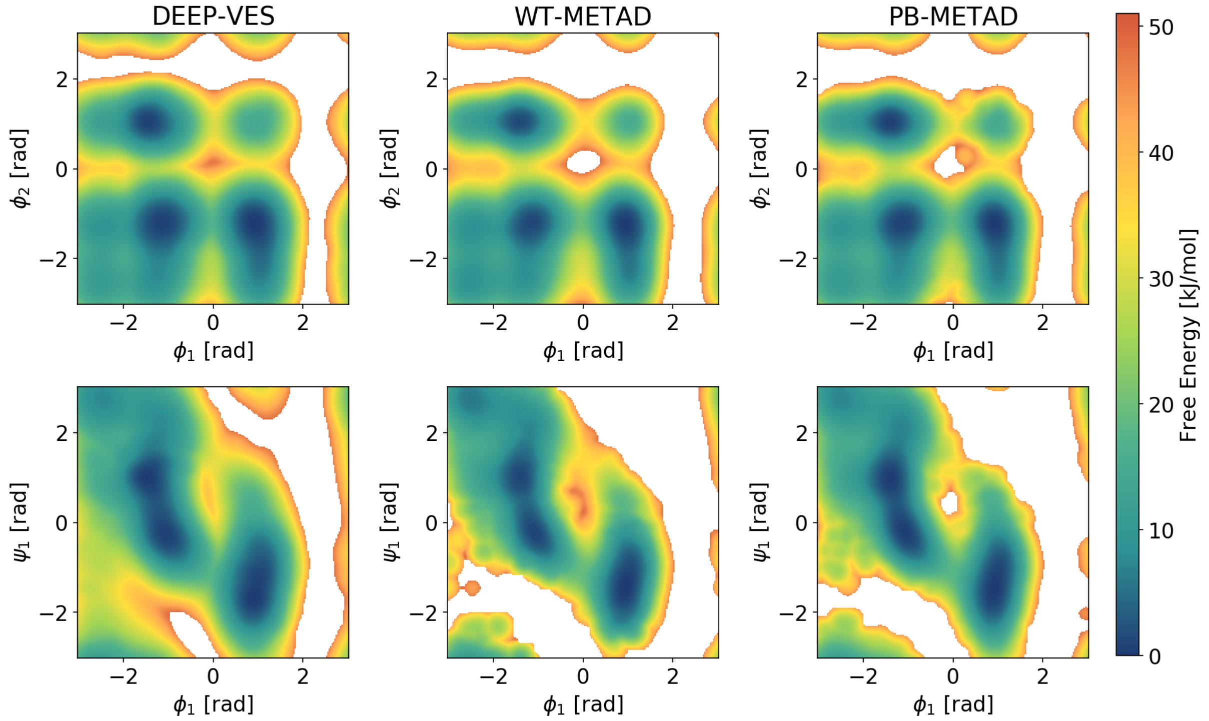


**Fig. S4.** Alanine tetrapeptide. Comparison of the free energy surfaces obtained by reweighting with the ones obtained with metadynamics and parallel-bias metadynamics. The regions of the FES greater than 50 kJ/mol are not shown.

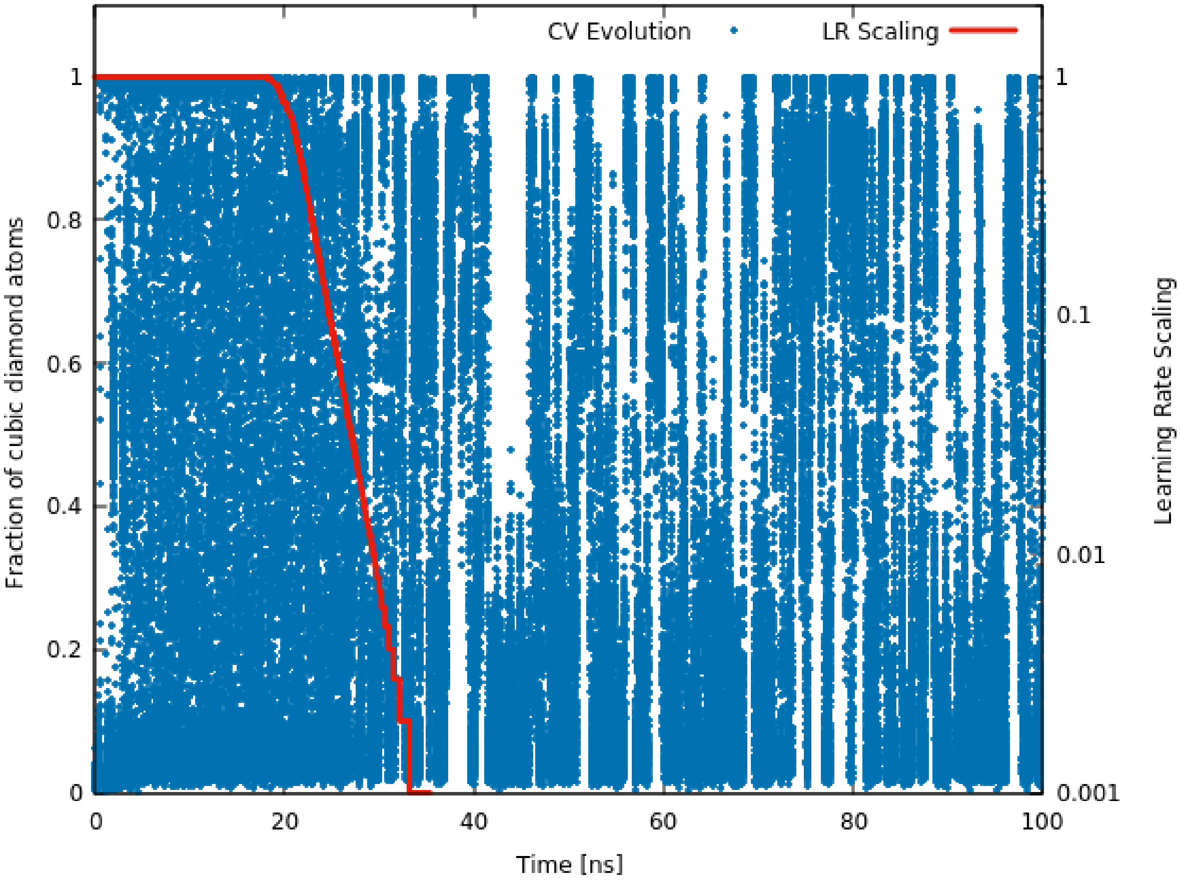


**Fig. S5.** Silicon crystallization. Fraction of cubic diamond atoms with respect to simulation time and scaling of the learning rate.
